# Supplementary material for: A Tale of Two Trees: One Writes, and Other Reads. Optimized Oblivious Accesses to Large-Scale Blockchains
Source: arXiv:1909.01531 source file (2019-09-16)
Supplement: Supplementary file 1 [file appendix.tex]

%!TEX root = main.tex
%
% \section{Appendix}
